# Supplementary material for: Froude number scaling unifies impact trajectories into granular media across gravitational conditions
Source: arXiv:2307.10998 source file (2023-07-20)
Supplement: Supplementary file 1 [file supp.tex]

\begin{document}

testing
\end{document}
